# Supplementary material for: A Moral Framework for Understanding of Fair ML through Economic Models of Equality of Opportunity
Source: arXiv:1809.03400 source file (2018-11-27)
Supplement: Supplementary file 1 [file appendix.tex]

\begin{figure}[h!]
    \centering
    \begin{subfigure}[b]{0.32\textwidth}
        \includegraphics[width=\textwidth]{Figures/group0_utility.png}
        \label{fig:util0}
    \end{subfigure}
    \begin{subfigure}[b]{0.32\textwidth}
        \includegraphics[width=\textwidth]{Figures/group1_utility.png}
        \label{fig:util1}
    \end{subfigure}
    \begin{subfigure}[b]{0.32\textwidth}
        \includegraphics[width=\textwidth]{Figures/group0_utility.png}
        \label{fig:util_wrong}
    \end{subfigure}
       \caption{The utility functions for groups 0 and 1. }
       \label{fig:utilities}
\end{figure}

\appendix

\section{Omitted Technical Material}\label{sec:technical}

\paragraph{Proof of Lemma~\ref{lem:represent}}
\begin{proof}
Solving the following system of equations,
\[ \forall y,\hy \in \{0,1\}: c^\vz_y \hy + d^\vz_y = b^\vz_{y,\hy}\]
we obtain: $c^\vz_0 = b^\vz_{0,1} - b^\vz_{0,0}$, $c^\vz_1 = b^\vz_{1,1} - b^\vz_{1,0}$, $d^\vz_0 = b^\vz_{0,0}$, and $d^\vz_1 = b^\vz_{1,0}$.
\end{proof}

\iffalse
\paragraph{Proof of Corollary~\ref{cor:d}}
\begin{proof}
Recall that we assumed $u^\vz(y,\hy) = \hy - g(\vx,y,\hy)$, or equivalently, 
$$g(\vz,y,\hy) = \hy - u^\vz(y,\hy).$$
Replacing $u^\vz(y,\hy)$ with the expression derived in Lemma~\ref{lem:represent}, we have:
\begin{eqnarray*}
g(\vz,y,\hy) &=&  \hy - \lbrace y \left(c^\vz_y \hy + d^\vz_y \right) + (1-y)\left(c^\vz_{1-y} \hy + d^\vz_{1-y}\right) \rbrace \\
&=&  \hy - \lbrace y \left(c^\vz_1 \hy + d^\vz_1 \right) + (1-y)\left(c^\vz_0 \hy + d^\vz_0\right) \rbrace \\
&=&  \hy - \lbrace y \left((b^\vz_{1,1} - b^\vz_{1,0}) \hy + b^\vz_{1,0} \right) + (1-y)\left( (b^\vz_{0,1} - b^\vz_{0,0}) \hy + b^\vz_{0,0}\right) \rbrace \\
&=&  \hy -  y \left((b^\vz_{1,1} - b^\vz_{1,0}) \hy + b^\vz_{1,0} \right) + (y-1)\left( (b^\vz_{0,1} - b^\vz_{0,0}) \hy + b^\vz_{0,0}\right) \\
&=&  \hy \left( 1 - b^\vz_{0,1} + b^\vz_{0,0} \right) + \hy y \left( b^\vz_{0,1} - b^\vz_{0,0}-b^\vz_{1,1} + b^\vz_{1,0}\right) + y \left( b^\vz_{0,0} - b^\vz_{1,0}\right) - b^\vz_{0,0}
\end{eqnarray*}
\end{proof}
\fi

\section{Omitted Experimental Details}\label{app:experiments}
In our experiments, we measured the following quantities:
\begin{itemize}
\item \textbf{Positive residual difference}\citep{calders2013controlling} is computed by taking the absolute difference of mean negative residuals across groups:
$$\left|\frac{1}{|G_1^+|} \sum_{i \in G_1} \max\{0,(\hat{y}_i- y_i)\}  - \frac{1}{|G_2^+|}\sum_{i \in G_2} \max\{0,(\hat{y}_i -y_i)\}\right|$$
\item \textbf{Negative residual difference}
\citep{calders2013controlling} is computed by taking the absolute difference of mean negative residuals across groups:
$$\left|\frac{1}{|G_1^-|} \sum_{i \in G_1} \max\{0,(y_i - \hat{y}_i)\}  - \frac{1}{|G_2^-|}\sum_{i \in G_2} \max\{0,(y_i - \hat{y}_i)\}\right|$$
\item \textbf{Average utility} or social welfare is computed by taking the average benefit of all individuals in the test data set:
$$\left|\frac{1}{|G_1^-|} \sum_{i \in G_1} \max\{0,(y_i - \hat{y}_i)\}  - \frac{1}{|G_2^-|}\sum_{i \in G_2} \max\{0,(y_i - \hat{y}_i)\}\right|$$
\end{itemize}
